# Supplementary material for: Fair Wrapping for Black-box Predictions
Source: arXiv:2201.12947 source file (2022-11-01)
Supplement: Supplementary file 1 [file main.tex]

\section{Proofs}

\subsection*{Proof of \cref{thm:cvar_to_l1}}

To prove the theorem, we use the ``robust representation'' given by \citet{ru13}.
\begin{theorem}[Robust Representation~\citep{ru13}] 
    \begin{equation}\label{eq:robust_representation}
        \cvar{\beta}(Z) = \sup_{Q \in \mathcal{Q}} \expect[Z Q],
    \end{equation}
    where \( \mathcal{Q} = \{ Q \mid 0 \leq Q \leq \nicefrac{1}{1 - \beta}, \expect{Q} = 1 \} \).
\end{theorem}

\begin{proof}
\end{proof}
