# Supplementary material for: Fair Wrapping for Black-box Predictions
Source: arXiv:2201.12947 source file (2022-11-01)
Supplement: Supplementary file 2 [file neutral-loss.tex]

\section{Neutral Loss} \label{sec-neutral-loss}

The condition of ``neutrality'' as presented in the main-text is better known as the condition of a loss being \emph{fair} \cite{rwID}. Notably, this fair loss condition is distinct from that of algorithmic fairness and the corresponding fairness criteria over, \emph{i.e.}, predictors. Reiterating the condition for a fair loss: \( \partialloss{1}(1) = \partialloss{-1}(0) = 0 \) and \( 0 = \min \partialloss{1} = \min \partialloss{-1} \). As such, we deliberately break convention and rename this condition as the ``neutrality'' of a loss: the condition can be summarized as the condition that correct prediction does give a loss (positive value) nor a gain (negative value), and thus is neutral in its response (zero value).
